# Supplementary material for: Ponimator: Unfolding Interactive Pose for Versatile Human-human Interaction Animation
Source: arXiv:2510.14976 source file (2025-10-16)
Supplement: Supplementary file 1 [file fig_contact_diverse.tex]

\begin{table*}
    \centering
    \footnotesize
    \setlength{\tabcolsep}{0.2em} % Adjust horizontal padding
    \resizebox{\linewidth}{!}{
        \begin{tabular}{c|cccc}

        {Interactive Pose} & 
        \multicolumn{4}{c}{{Interaction Animation (left$\rightarrow$right: time steps)}} \\

    \includegraphics[width=0.2\linewidth]{rebuttal_src_figs/pair00_000040_1_10/00_crop.pdf} &
     \includegraphics[width=0.2\linewidth]{rebuttal_src_figs/pair00_000040_1_10/05_crop.pdf} &
      \fcolorbox{green}{white}{
      \includegraphics[width=0.2\linewidth]{rebuttal_src_figs/pair00_000040_1_10/10_crop.pdf}} & 
      \includegraphics[width=0.2\linewidth]{rebuttal_src_figs/pair00_000040_1_10/15_crop.pdf} &
      \includegraphics[width=0.2\linewidth]{rebuttal_src_figs/pair00_000040_1_10/19_crop.pdf} \\

    \includegraphics[width=0.2\linewidth]{rebuttal_src_figs/pair00_000040_1_20/05_crop.pdf} &
     \includegraphics[width=0.2\linewidth]{rebuttal_src_figs/pair00_000040_1_20/12_crop.pdf} &
      \includegraphics[width=0.2\linewidth]{rebuttal_src_figs/pair00_000040_1_20/15_crop.pdf} & 
      \fcolorbox{green}{white}{
      \includegraphics[width=0.2\linewidth]{rebuttal_src_figs/pair00_000040_1_20/20_crop.pdf}} &
      \includegraphics[width=0.2\linewidth]{rebuttal_src_figs/pair00_000040_1_20/23_crop.pdf} \\

    \end{tabular}
    }
\captionof{figure}{\textbf{Diverse interactive pose animation}. Given an interactive pose, we can synthesize different windows of past and future frames by adjusting the interactive time.}
\label{fig:exp-contact-diverse}
\end{table*}
